# Supplementary material for: ImpDet: Exploring Implicit Fields for 3D Object Detection
Source: arXiv:2203.17240 source file (2022-03-31)
Supplement: Supplementary file 1 [file tab_ablation_iarg_supp.tex]

\begin{table*}[tbh]
\begin{centering}
\small{
\setlength{\tabcolsep}{2.5mm}{
\begin{tabular}{c|ccc|ccc|ccc|ccc}
\hline
\multirow{3}{*}{Method} & \multicolumn{6}{c|}{\textit{centrosymmetry}} & \multicolumn{6}{c}{\textit{supplement}} \\
\cline{2-13} 
& \multicolumn{3}{c|}{point} & \multicolumn{3}{c|}{point+virtual} & \multicolumn{3}{c|}{point} & \multicolumn{3}{c}{point+virtual} \\
& Easy & Mod. & Hard & Easy & Mod. & Hard & Easy & Mod. & Hard & Easy & Mod. & Hard \\ \hline
$\rm AP_{3D}$ & 79.11 & 76.67 & 75.66 & 88.37 & 83.81 & 77.49 & 60.25 & 59.56 & 51.84 & 89.13 & 84.93 & 78.70 \\
$\rm AP_{BEV}$ & 86.39 & 85.62 & 79.07 & 89.74 & 87.93 & 87.25 & 69.89 & 61.96 & 53.40 & 90.27 & 88.00 & 88.63 \\ \hline
\end{tabular}}}
\par\end{centering}
\caption{Comparison of different segmentation boundary generation algorithms on KITTI \textit{val} set with mAP calculated by 11 recall positions for car class. 
\label{Tab: Ablation_IARG_supp}}
\end{table*}
